# Supplementary material for: Accelerated Multiplicative Weights Update Avoids Saddle Points almost always
Source: arXiv:2204.11407 source file (2022-04-25)
Supplement: Supplementary file 1 [file supplementary.tex]

%%%% ijcai22.tex

\typeout{IJCAI--22 Instructions for Authors}

% These are the instructions for authors for IJCAI-22.

\documentclass{article}
\pdfpagewidth=8.5in
\pdfpageheight=11in
% The file ijcai22.sty is NOT the same as previous years'
\usepackage{ijcai22}

% Use the postscript times font!
\usepackage{times}
\usepackage{soul}
\usepackage{url}
\usepackage[hidelinks]{hyperref}
\usepackage[utf8]{inputenc}
\usepackage[small]{caption}
\usepackage{graphicx}
\usepackage{amsmath}
\usepackage{amsthm}
\usepackage{booktabs}
\usepackage{algorithm}
\usepackage{algorithmic}
\usepackage{amsfonts}    
\urlstyle{same}

\usepackage{nccmath}

\usepackage[utf8]{inputenc} % allow utf-8 input
\usepackage[T1]{fontenc}    % use 8-bit T1 fonts
\usepackage{hyperref}       % hyperlinks
\usepackage{amsthm}
\usepackage{amsmath}
\usepackage{url}            % simple URL typesetting
\usepackage{booktabs}       % professional-quality tables
\usepackage{amsfonts}       % blackboard math symbols
\usepackage{nicefrac}       % compact symbols for 1/2, etc.
\usepackage{microtype}      % microtypography
\usepackage{xcolor}         % colors
\usepackage{array}
\usepackage{subfigure}
\usepackage{graphicx}
\usepackage{tikz}
\usepackage{pgf, tikz}
\usetikzlibrary{arrows, automata}
\usepackage{comment}
\usepackage[skins]{tcolorbox}
\usepackage{algorithm}
\usepackage{algorithmic}

% the following package is optional:
%\usepackage{latexsym}

% See https://www.overleaf.com/learn/latex/theorems_and_proofs
% for a nice explanation of how to define new theorems, but keep
% in mind that the amsthm package is already included in this
% template and that you must *not* alter the styling.

\usepackage{xcolor}
\usepackage{pgfplots}
\usepackage{mathtools}

\usepackage{xr}
\externaldocument{ijcai22}

\providecommand{\customgenericname}{}
\newcommand{\newcustomtheorem}[2]{%
  \newenvironment{#1}[1]
  {%
   \renewcommand\customgenericname{#2}%
   \renewcommand\theinnercustomgeneric{##1}%
   \innercustomgeneric
  }
  {\endinnercustomgeneric}
}

\newcustomtheorem{customthm}{Theorem}
\newcustomtheorem{customlemma}{Lemma}

 % No op here. Customize it for different styles.

%\DeclarePairedDelimiter{\norm}{\lVert}{\rVert}

% Following comment is from ijcai97-submit.tex:
% The preparation of these files was supported by Schlumberger Palo Alto
% Research, AT\&T Bell Laboratories, and Morgan Kaufmann Publishers.
% Shirley Jowell, of Morgan Kaufmann Publishers, and Peter F.
% Patel-Schneider, of AT\&T Bell Laboratories collaborated on their
% preparation.

% These instructions can be modified and used in other conferences as long
% as credit to the authors and supporting agencies is retained, this notice
% is not changed, and further modification or reuse is not restricted.
% Neither Shirley Jowell nor Peter F. Patel-Schneider can be listed as
% contacts for providing assistance without their prior permission.

% To use for other conferences, change references to files and the
% conference appropriate and use other authors, contacts, publishers, and
% organizations.
% Also change the deadline and address for returning papers and the length and
% page charge instructions.
% Put where the files are available in the appropriate places.

% PDF Info Is REQUIRED.
% Please **do not** include Title and Author information
%\pdfinfo{
%/TemplateVersion (IJCAI.2022.0)
%}

\title{IJCAI--22 Formatting Instructions}

% Single author syntax

% Multiple author syntax (remove the single-author syntax above and the \iffalse ... \fi here)
% Check the ijcai22-multiauthor.tex file for detailed instructions

\author{
First Author$^1$
%\and
%Second Author$^2$\and
%Third Author$^{2,3}$\And
%Fourth Author$^4$
\affiliations
$^1$First Affiliation\\
%$^2$Second Affiliation\\
%$^3$Third Affiliation\\
%$^4$Fourth Affiliation
\emails
\{first, second\}@example.com,
third@other.example.com,
fourth@example.com
}

\begin{document}

%\maketitle

\onecolumn

%Multiplicative Weights Update (MWU) has beed studied extensively due to many applications in constrained optimization, game theory, and machine learning. Despite the popularity of the algorithm, there are two questions remain unaddressed: (1) whether there is an accelerated version of MWU, and (2) whether there is a perturbed version of MWU so that the efficiency in escaping saddle points can be discussed. This paper focuses on a spherical framework for MWU, i.e., MWU is formulated as a manifold gradient descent. We provide two important applications of this approach: acceleration and non-asymptotic convergence. As for the accelerated MWU, we prove that it converges to second-order stationary points almost always, and for the perturbed MWU, we show that the efficiency in escaping saddle points fits into the framework of perturbed Riemannian gradient descent.

%\input{experiment}

\input{appendix}

\bibliographystyle{plain}
\bibliography{Bibli}

%\bibliographystyle{named}
%\bibliography{ijcai22}

\end{document}
